# Supplementary material for: Uncertainty-Induced Transferability Representation for Source-Free Unsupervised Domain Adaptation
Source: arXiv:2208.13986 source file (2022-08-30)
Supplement: Supplementary file 1 [file supplement.tex]

\section{Extra Study}
\label{sup_sec1}
\noindent \textbf{Implementation details.} 
In the Section 3.2 of the main submission, we prove that the domain distributional representation uncertainty $DDRU(h_s)$  reveals the transferability of the source features on three Office-Home adaptation tasks: $Cl\rightarrow Ar$, $Cl\rightarrow Pr$ and $Cl\rightarrow Re$.
In the following, we conduct more experiments to study the $DDRU(h_s)$.

We adopt the backbone of ResNet-50 \cite{he2016deep} (for office-31 and office-home) or ResNet-101 (for VisDA) along with a fully-connected (FC) ($\mathbb{R}^ {2048 \times 256}$) layer as the feature encoder, and a FC layer  with a weight normalization layer as the classifier.
Following \cite{liang2020we,yang2021exploiting}, the source model is trained by the cross-entropy loss with the label smoothing (LS) technique \cite{muller2019does}.
The target classifier is initialized with the source domain parameters and fixed during the adaptation.
We adopt SGD with momentum 0.9 and batch size of 64 on all datasets. 
For the Office-31 and Office-home datasets, the learning rate of the ResNet-50 backbone and the newly added layers are 1e-3 and 1e-2 respectively. The learning rate is 1e-4 for VisDA. We train 20, 30 and 15 epochs for Office-31, Office-Home and VisDA respectively. 
The threshold of IRI $\tau_{r}$ are set to be 3 times of the mean of target samples' IRI, i.e. $\tau_{r}=3*\frac{1}{n_t}\sum_{i=1}^{n_t}IRI(x_t^i)$, which is updated during each epoch. For the uncertainty measurement, we perform $T=2$ perturbations, each of which $r_t$ is randomly sampled from $U(-0.05,0.05)$.
We set the hyper-parameter $\lambda_1$ of the transferability-induced knowledge distillation loss $\lambda_1=10$ at the beginning and after 10 epochs $\lambda_1=0$. The hyper-parameter $\lambda_2$ of the forget loss is 0.9. The MMD \cite{gretton2006kernel}, A-distance \cite{ben2010theory}, Corresponding Angle \cite{chen2019transferability}, LogME \cite{you2021logme}, LEEP \cite{nguyen2020leep} ,NCE\cite{tran2019transferability} and the prediction accuracy are used as the criterion to measure the transferability. Following the Section 5, we split the 256-dim representations $z=h_s(x)$ into two separate 128-dim vectors $z_{low}$ and $z_{high}$, representing the ones with the 128 smallest $DDRU^i(h_s)$ and the 128 largest $DDRU^i(h_s)$ respectively. We conduct the above measurements on the $z_{low}$ and $z_{high}$ respectively, to evaluate the consistency of DDRU with these measurements.

\noindent \textbf{Experiment Setting.} 
First, we have demonstrated the effectiveness of $DDRU$ on three Office-Home adaptation tasks: $Cl\rightarrow Ar$, $Cl\rightarrow Pr$ and $Cl\rightarrow Re$ in the Section 3.3 of the main submission. Here, we investigate the effectiveness of DDRU on more tasks, including the VisDA tasks (Figure \ref{fig:visda}), the Office-31 tasks (Figure \ref{fig:31}), and the rest Office-home tasks (Figure \ref{fig:home})

Second, in our previous experiments, $DDRU(h_s)$ is calculated using the last layer output of the feature extractor (the FC layer). Here, we explore the feasibility of extending the DDRU to feature representation of other layers. To this end, we use the average pooling to extract features $z \in \mathbb{R}^ {2048}$ from the last, penultimate, and antepenultimate bottleneck of the Resnet50 backbone, respectively. 
Then we calculate the DDRU $DDRU(h_s)$ of these features and evaluate its effectiveness. The evaluation method is similar to the previous one: that is, the feature $z$ is divided into two 1024-dimension vectors  $z_{low}$ and $z_{high}$ according to $DDRU(h_s)$, and their corresponding angles are compared to evaluate their transferability. The results are shown in Figure \ref{fig:corrlayer}.

\begin{figure}[t]
  \centering
  %\fbox{\rule{0pt}{2in} \rule{0.9\linewidth}{0pt}}
 
    \includegraphics[width=0.8\linewidth]{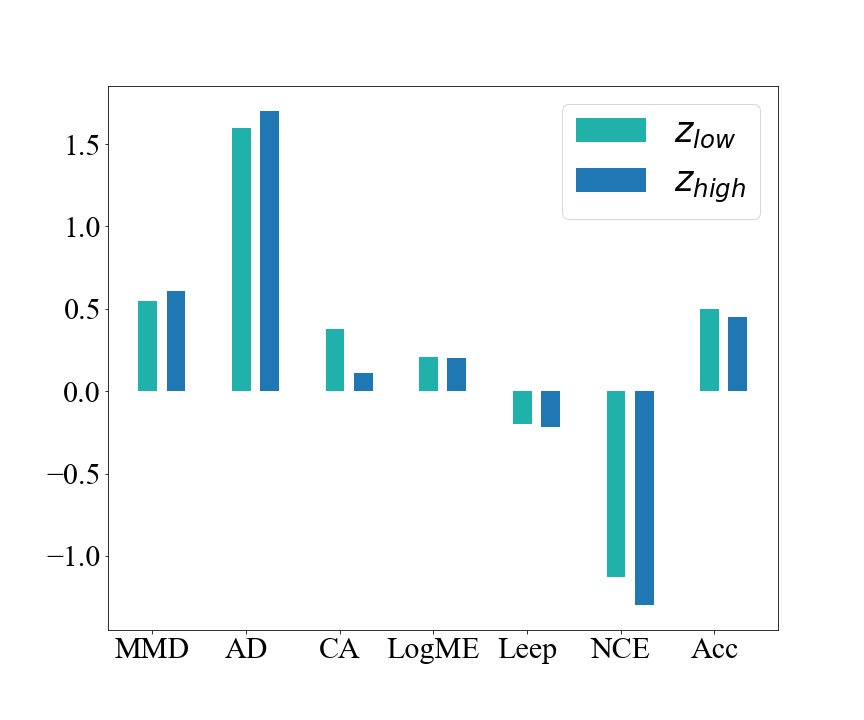}

   \caption{  The consistency of the DDRU and current transerability measurements (MMD, A-distance (AD), Corresponding Angle(CA), LogME, LEEP, NCE and the prediction accuracy) on VisDA task(synthetic$\rightarrow$real).
   $z_{low}$ and $z_{high}$   represent the dimensions with the 128 smallest $DDRU^i(h_s)$ and the 128 largest $DDRU^i(h_s)$ respectively. 
   }
   \label{fig:visda}
\end{figure}

\begin{figure*}[t]
  \centering
     \subfigure[]{
    \includegraphics[width=0.25\linewidth]{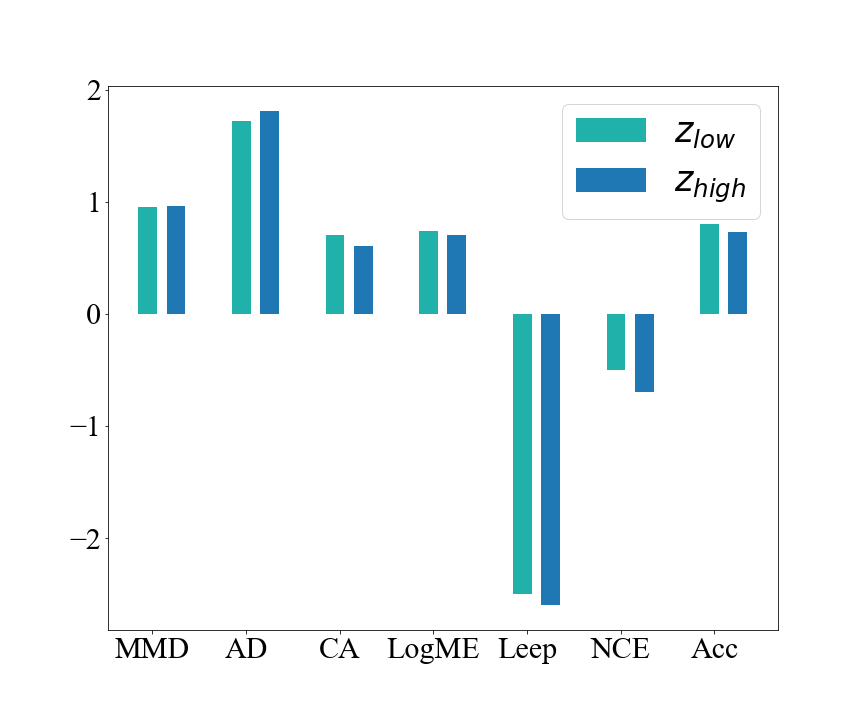}}
     \subfigure[]{
    \includegraphics[width=0.25\linewidth]{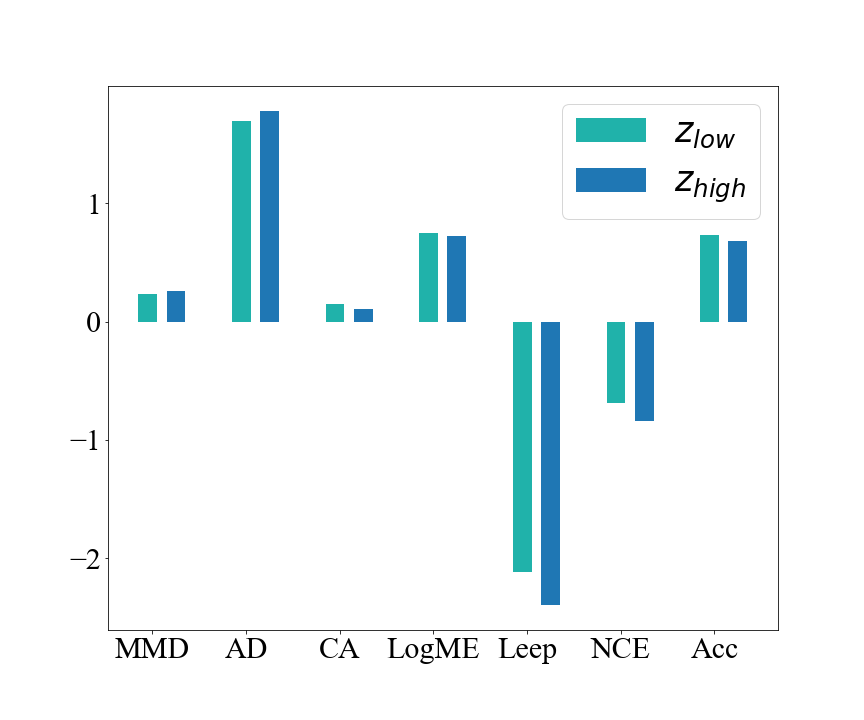}}
    \subfigure[]{
    \includegraphics[width=0.25\linewidth]{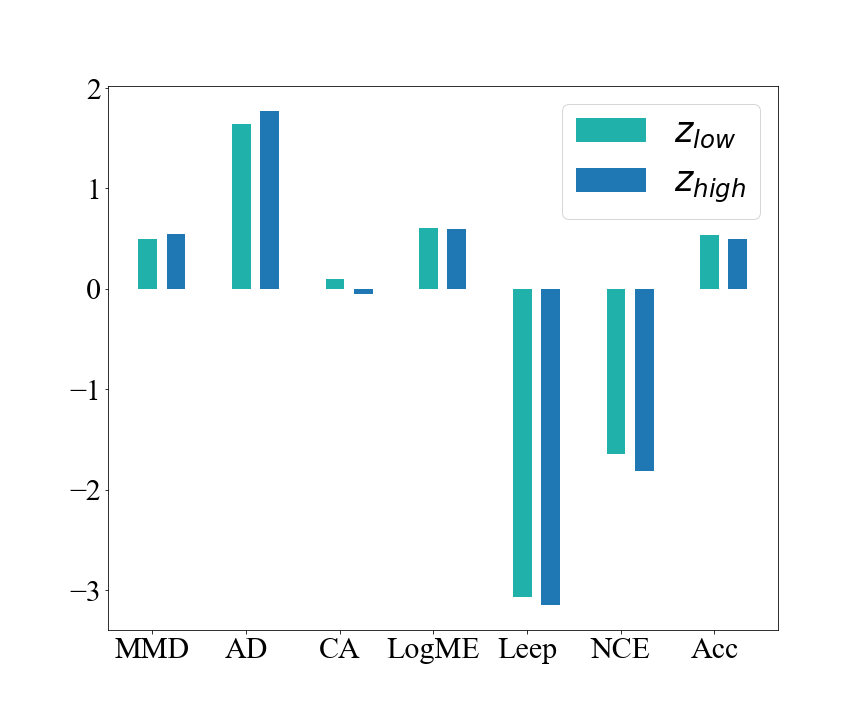}
    }
    
     \subfigure[]{
    \includegraphics[width=0.25\linewidth]{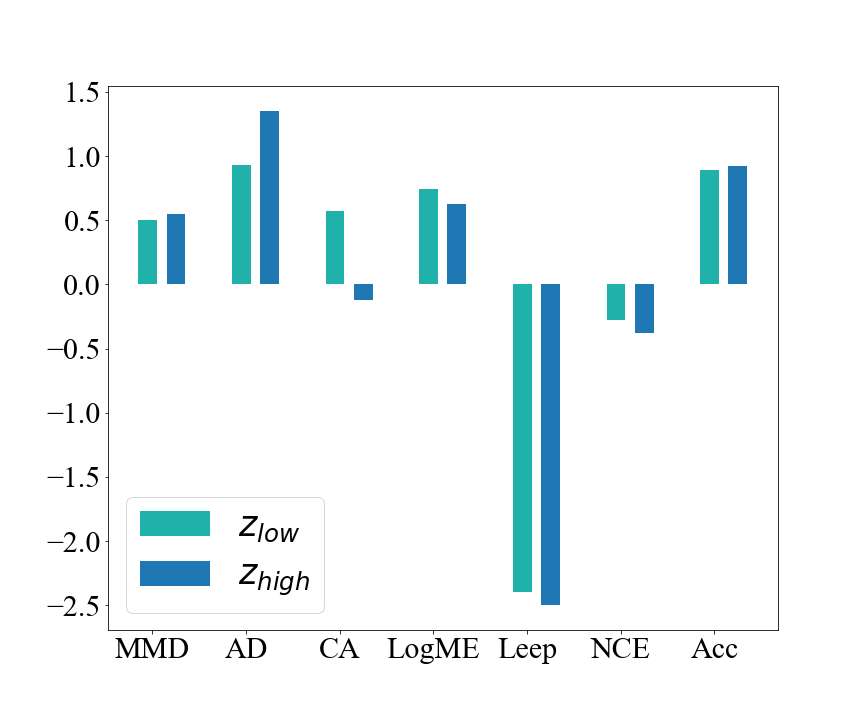}}
     \subfigure[]{
    \includegraphics[width=0.25\linewidth]{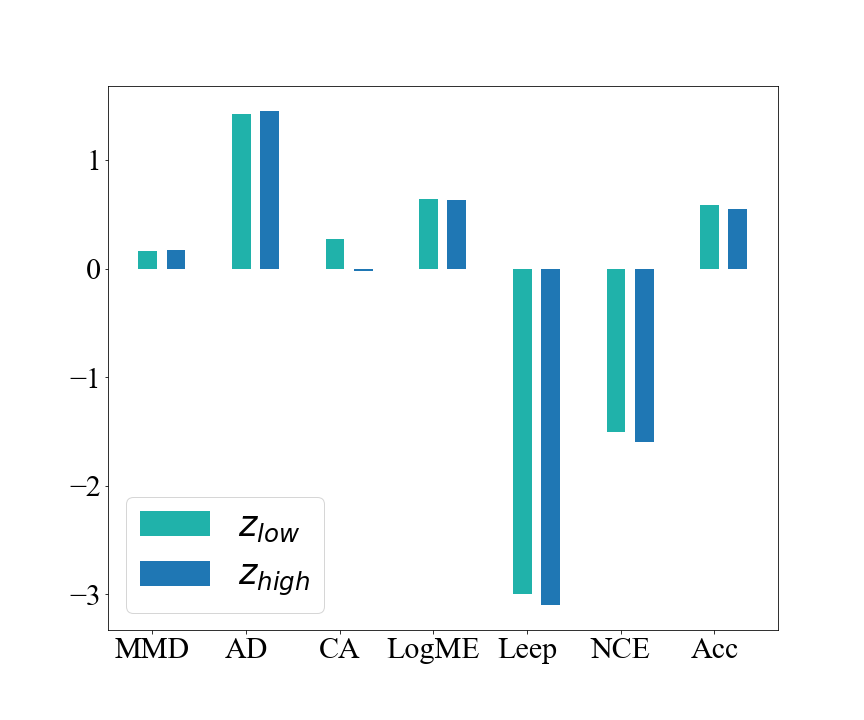}}
    \subfigure[]{
    \includegraphics[width=0.25\linewidth]{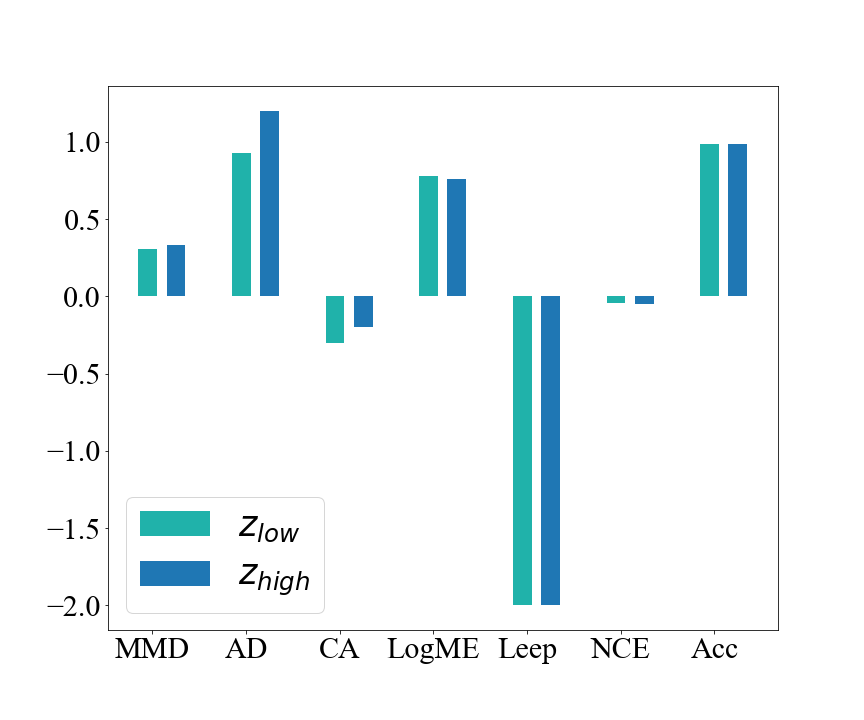}
    }
    \vspace{-2mm}
   \caption{  The consistency of the DDRU and current transerability measurements (MMD, A-distance (AD), Corresponding Angle(CA), LogME, LEEP, NCE and the prediction accuracy) on Office-31 tasks.
   $z_{low}$ and $z_{high}$   represent the dimensions with the 128 smallest $DDRU^i(h_s)$ and the 128 largest $DDRU^i(h_s)$ respectively. }
   \label{fig:31}
\end{figure*}

Third, we have investigated the effectiveness of our DDRU on the source model,  now we evaluate it on the target model in the adaptation process. 
Following the previous Section 3.2 in the main submission, we split the features $z$ extracted by the target model into two separate 128-dim vectors $z_{low}$ and $z_{high}$, representing the ones with the 128 smallest $DDRU^i(h_s)$ and the 128 largest $DDRU^i(h_s)$ respectively. Then the corresponding angle is used to evaluate the transferability of the $z_{low}$ and $z_{high}$. The results of the model adapted with 5, 10, 15, 20, 25 and 30 epochs are shown in Figure \ref{fig:epoch}.

\input{tables/tab_tran_others}
%\begin{figure*}[t]
%  \centering
    
%    \includegraphics[width=0.9\linewidth]{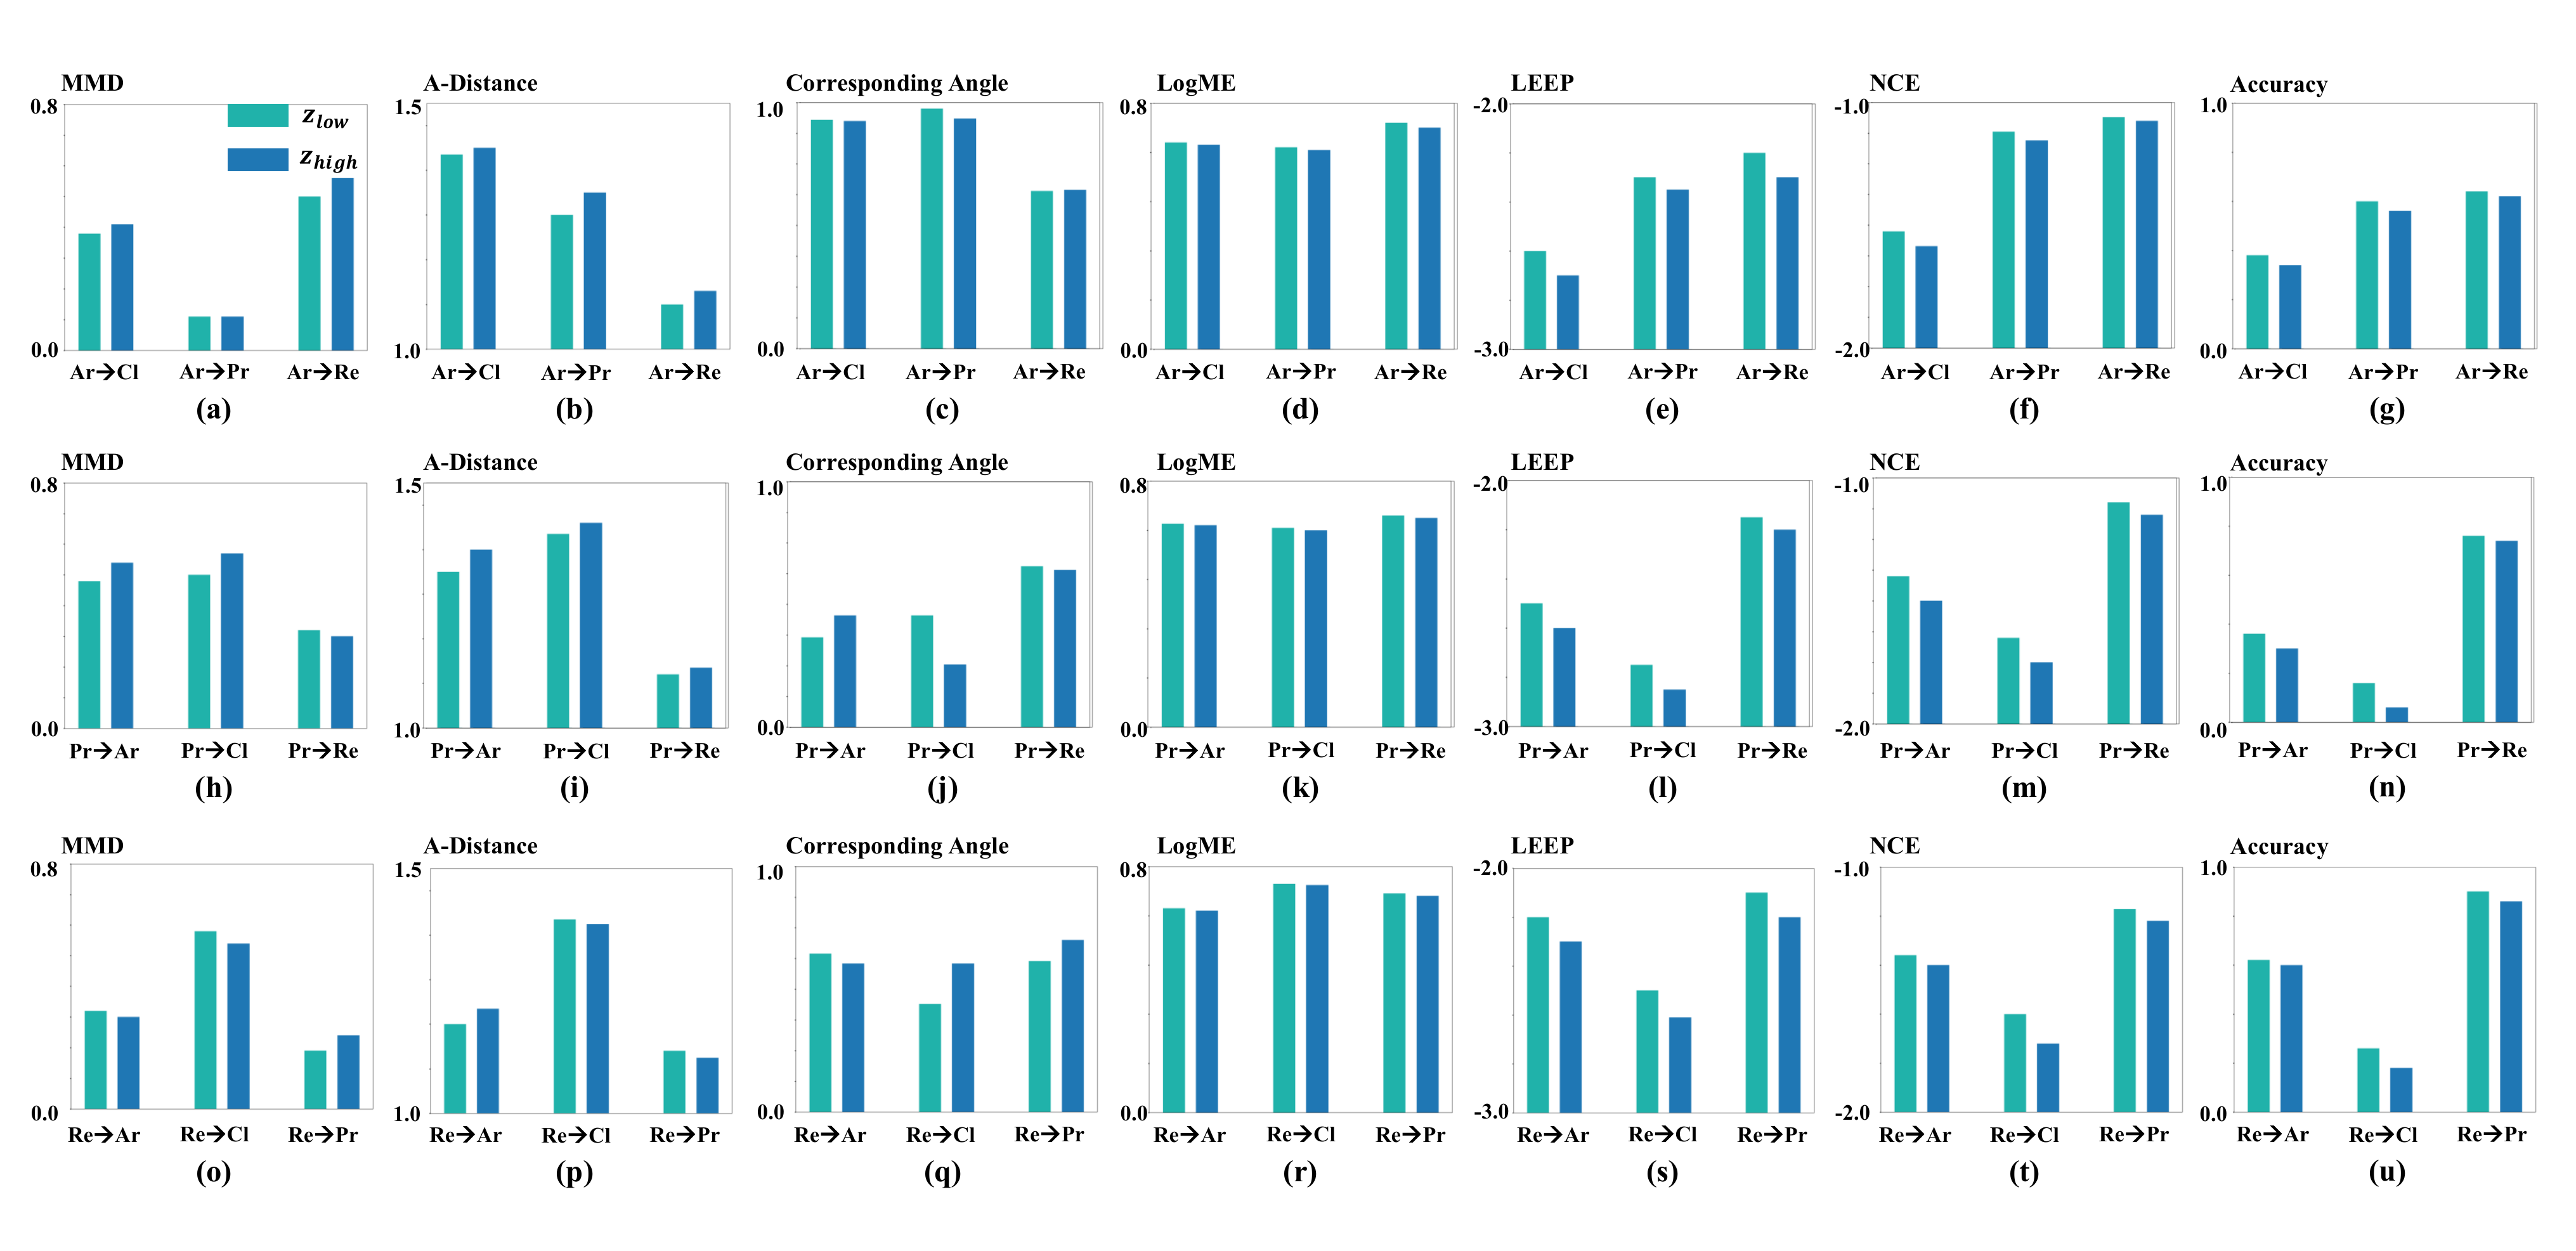}
 %  \caption{ The consistency of the DDRU and current transerability measurements (MMD, A-distance (AD), Corresponding Angle(CA), LogME, LEEP, NCE and the prediction accuracy) on Office-home tasks. $z_{low}$ and $z_{high}$   represent the dimensions with the 128 smallest $DDRU^i(h_s)$ and the 128 largest $DDRU^i(h_s)$ respectively.}
%   \label{fig:home}
%\end{figure*}

\begin{figure*}[t]
  \centering
   \subfigure[]{
    \includegraphics[width=0.25\linewidth]{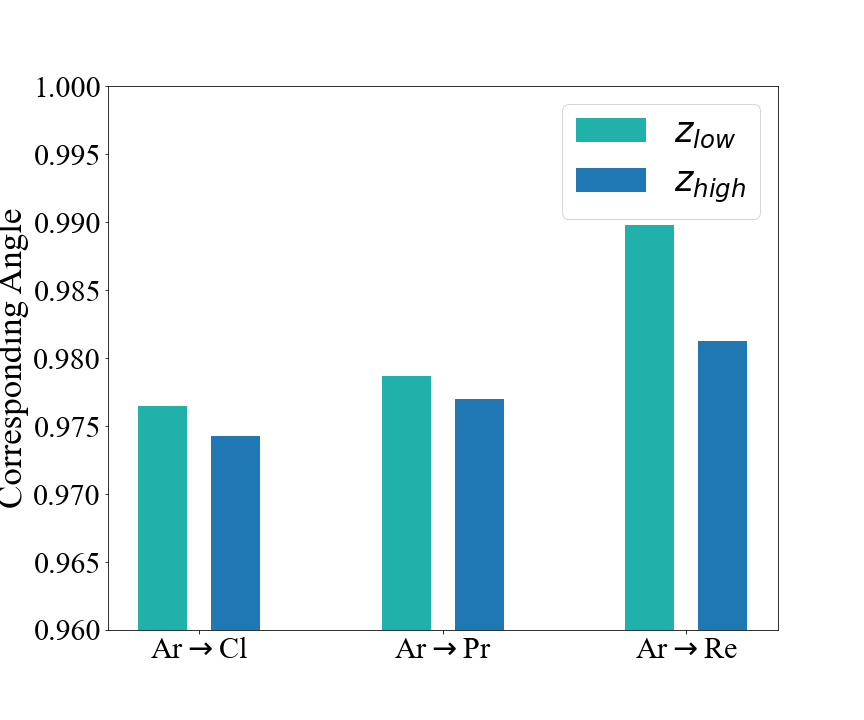}}
     \subfigure[]{
    \includegraphics[width=0.25\linewidth]{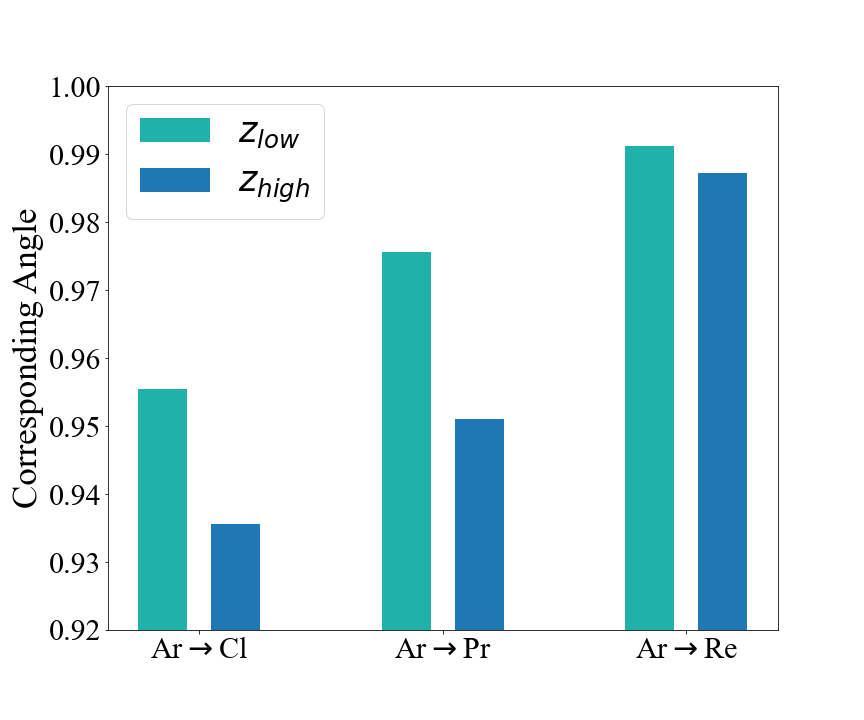}}
     \subfigure[]{
    \includegraphics[width=0.25\linewidth]{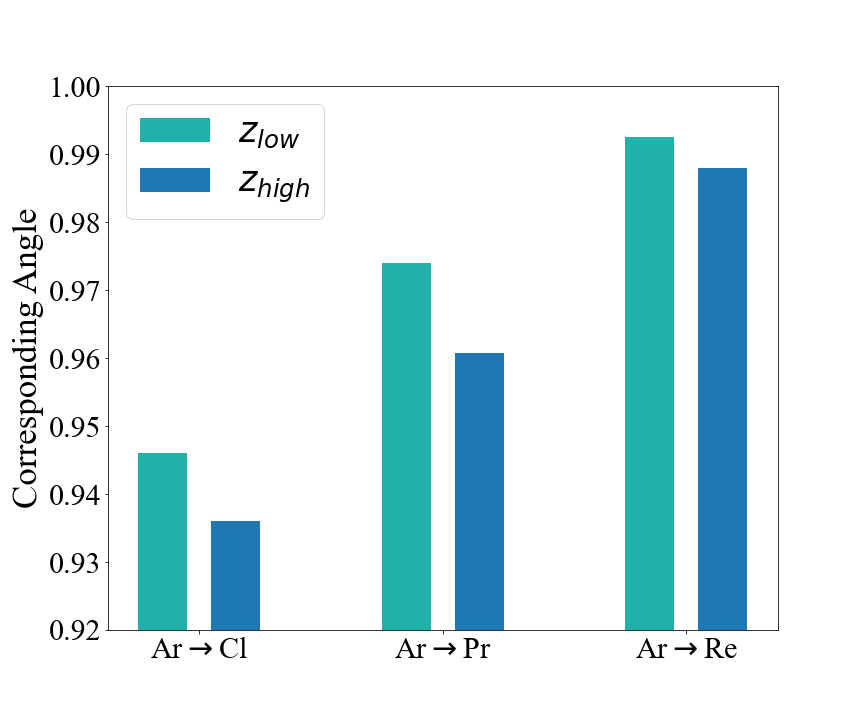}}
   \caption{ The effectiveness of the DDRU for features extracted at different layers. (a): At the last layer. (b) At the penultimate layer. (c) At the antepenultimate layer.}
   \label{fig:corrlayer}
\end{figure*}

\begin{figure*}[t]
  \centering
     \subfigure[]{
    \includegraphics[width=0.25\linewidth]{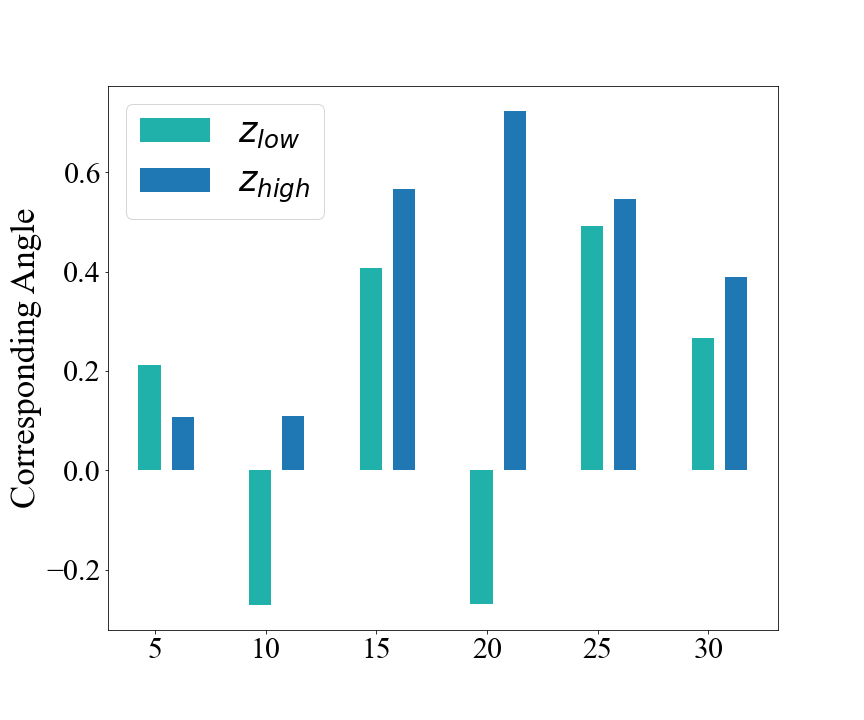}}
     \subfigure[]{
    \includegraphics[width=0.25\linewidth]{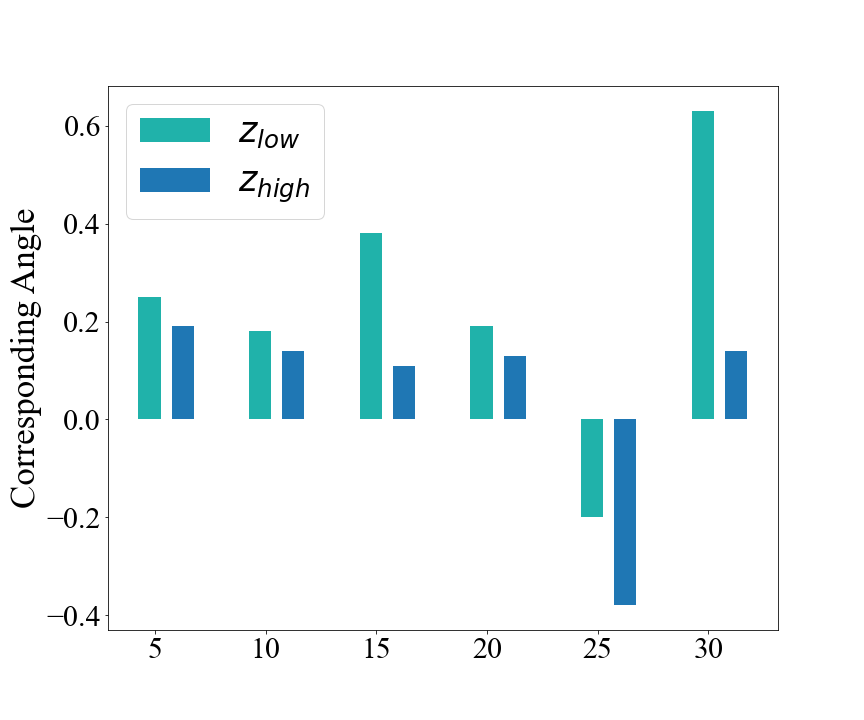}}
    \subfigure[]{
    \includegraphics[width=0.25\linewidth]{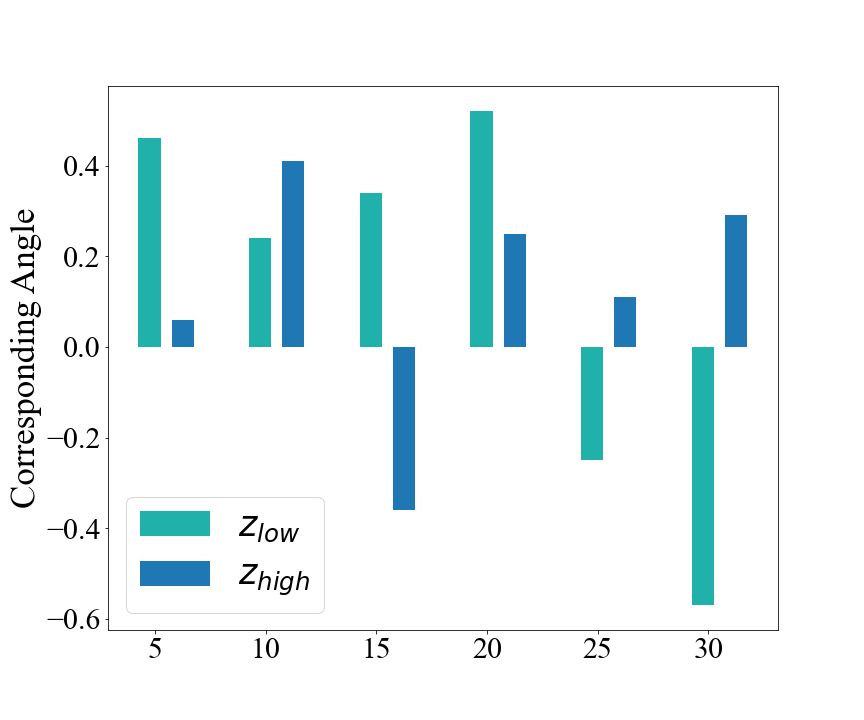}
    \label{fig:1c}
    }
    \vspace{-2mm}
   \caption{ The effectiveness of the DDRU in the adaptation process. $z_{low}$ and $z_{high}$   represent the dimensions with the 128 smallest $DDRU^i(h_s)$ and the 128 largest $DDRU^i(h_s)$ respectively. The larger corresponding angle indicates that the features are more transferable. The adaptation results trained with 5, 10, 15, 20, 25 and 30 epochs are reported.}
   \label{fig:epoch}
\end{figure*}

\noindent \textbf{The effectiveness of DDRU.}
We evaluate the effectiveness of DDRU on the VisDA tasks, the Office-31 tasks, and the rest Office-home task. From Figure \ref{fig:visda}, we can see that DDRU is consistent \lisays{with} previous measurements on the VISDA. Specifically, $z_{low}$ that with low DDRU, producing low MMD and \mathcal{A}-Distance between source and target domain than $z_{high}$, which illustrates that $z_{low}$ is effective in eliminating the discrepancy between the source and target domain. 
It can also be seen that in terms of the Corresponding Angle, LogME, LEEP, NCE, and the prediction accuracy, $z_{low}$ is higher than $z_{high}$, which proves the consistency between DDRU and these measurements.
In particular, the prediction accuracy of $z_{low}$ on the target domain is 50.7\%, which is significantly superior \lisays{to} $z_{high}$ that only achieves 45.5\%, which directly demonstrates that $z_{low}$ is more transferable to target domain than  $z_{high}$.
These phenomenons can be observed in most Office-31 tasks (Figure \ref{fig:31}) and Office-home tasks  (Figure \ref{fig:home}). The experimental observations from the series of studies above illustrate the proposed DDRU is strongly consistent with current transferability measurements in most cases; thus, it can estimate the transferability.

\noindent \textbf{Extension to other layers.}
We explore the feasibility of extending the DDRU to feature representation of other layers on three office-home tasks: $Ar\rightarrow Cl$, $Ar\rightarrow Pr$ and $Ar\rightarrow Re$.
We calculated the DDRU on the last, penultimate, and antepenultimate bottleneck of the Resnet50 backbone, respectively. 
From Figure \ref{fig:corrlayer}, it can be seen that the corresponding angle of features $z_{low}$ with lower DDRU, is larger than $z_{high}$ with higher DDRU. Therefore, the DDRU is effective for identifying other layers' features as well, including the last, penultimate, and antepenultimate bottleneck of Resnet-50. The similar trends among multiple layers' features proves that our transferable index has the potential to extend to feature representation of other layers.

\noindent \textbf{DDUR in the adaptation process.} 
The above experiments prove favourably that the DDRU can be used to estimate the transferability of the source model. 
From figure \ref{fig:epoch}, we can see that DDRU is also effective to the target model in the first few steps of adaptation. To be specific, we can see that in the first 5 \lisays{steps}, the $z_{low}$ has \lisays{a} larger Corresponding Angle between the source domain and the target domain than $z_{high}$, which indicates that it is more transferable between the two domains.
However, it can be seen that after  training for a period, it is inadequate to use the DDRU for identifying the target model. 
For example, in the epoch 10/30 of Figure \ref{fig:1c}, the corresponding angle of $z_{low}$ is lower than $z_{high}$. 
This phenomenon indicates that after a period of training, the target model gradually adapts to the target domain. Thus, it no longer needs and even actively abandons the source model knowledge, which makes the DDRU invalid.
This is why we terminate the "inherit" step after 10 \lisays{epochs} with $\lambda_1 =0$.
